# Supplementary material for: Tunable spin and orbital Edelstein effect at (111) LaAlO$_3$/SrTiO$_3$ interface
Source: arXiv:2207.07663 source file (2022-07-15)
Supplement: Supplementary file 2 [file Supplementary_old.tex]

\clearpage
\onecolumngrid
\section{Single band model}
In a simple generalized Rashba model the spectra for low fillings can be written as a quadratic function of $\vec{k}$ and a $|\vek|$ dependent Rashba coefficient as
\begin{equation}
    \varepsilon_\sigma(|\vek|)=\frac{\beta}{2}k^2+\alpha(|\vek|)\sigma.
\end{equation}
It can be proved by explicitly make the integral~\ref{chi} that the magnetic moment is proportional to the energy splitting between the states with different spin as
\begin{equation}
    m\propto\frac{2\alpha(|\vek|)}{\beta |\vek|}.
\end{equation}
In this framework, we show in Fig.~\ref{splitting12} the energy splitting of the first two bands of the complete model as a function of $|\vek|$ and observe that a structure similar to the single doublet curves in Fig.~\ref{fig:Edelstein_chi}.
\begin{figure}[t!]
    \centering
    \includegraphics[width=0.45\textwidth]{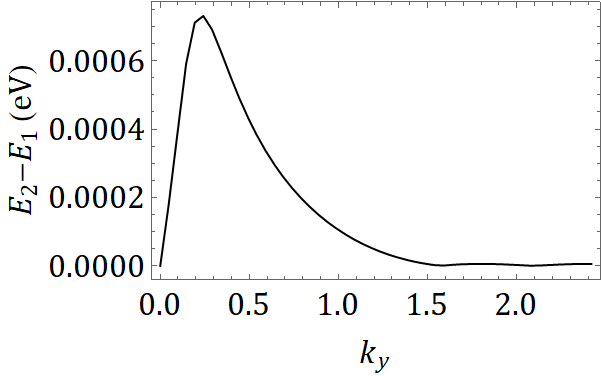}
    \caption{}
    \label{splitting12}
\end{figure}
Moreover, by inverting the relation between $\varepsilon$ and $\vek$, one can find that the peak of the red curve in Fig.~\ref{fig:Edelstein_chi}(a) is located approximately to the same fillings. However, there are some feature that are not captured by this model: the different sign of the Rashba coefficients for the second doublet has no explanation in a simple model, and the second doublet has no linear splitting and so this model is not suitable for explaining this structure. Moreover all the three curves does not saturates to zero, but to a finite constant, even changing sign with the filling.
This simple framework can explain approximately the first peak of the red curve of $\chi^S$, but diverges when more bands are filled. That even taking three different isolated bands with Rashba splitting cannot reproduce the results. 
